# Supplementary material for: A study of events with photoelectric emission in the DarkSide-50 liquid argon Time Projection Chamber
Source: arXiv:2107.08015 source file (2021-11-27)
Supplement: Supplementary file 1 [file Supplemental_Material.tex]

\section{Pathological Events}
\label{sec:Appendix_Pathological}
Among the events that have been analysed in the manuscript, some of them turned out to have some strange behaviour, for which they have not been understood and categorized thoroughly. In particular, we are referring to the vertical population in fig. \ref{fig:SEC-S2} distributed between $350 \mus <\Delta t_{\mathrm{SEC}-\mathrm{S2}}<375 \mus$. 
\begin{figure}
\begin{center}
\includegraphics[width=\columnwidth]{Final_figures/Pathological_Events.pdf}
\caption{Distribution of the time difference $\Delta t_{\mathrm{SEC}-\mathrm{S2}}$ vs. the time difference $\Delta t_{\mathrm{SEC}-\mathrm{S1}}$ for events with  SEC amplitude $>$70 PE.}
\label{fig:Pathological_Events}
\end{center}
\end{figure}
In fig. \ref{fig:Pathological_Events} the distribution of time requiring a SEC amplitude $>70$ PE is shown. It is visible that the majority of events is represented by S1-echo (the vertical strip at $\Delta t_{\mathrm{SEC}-\mathrm{S1}}\sim 380 \mus$), S2-echo (the horizontal strip corresponding to $\Delta t_{\mathrm{SEC}-\mathrm{S2}}\sim 380 \mus$) and the events gathered on the top-right region of the plot. As a reference, the diagonal of the plot indicates $\Delta t_{\mathrm{S2}-\mathrm{S1}}=0$), so that events close to the diagonal have been generated by interactions happened near the top of the TPC. The origin of this set of events has not a clear explanation, so it needs to be further investigated in future analyses.
